# Supplementary material for: DUET: A Tuning-Free Device-Cloud Collaborative Parameters Generation Framework for Efficient Device Model Generalization
Source: arXiv:2209.05227 source file (2024-12-01)
Supplement: Supplementary file 1 [file 9appendix.tex]

\appendix

\section{Appendix}
\label{sec:appendix}
This is the Appendix for ``DUET: A Tuning-Free Device-Cloud Collaborative Parameters Generation Framework for Efficient Device Model Generalization''.

\begin{itemize}

\item Section ~\ref{sec:appendix_limitation_of_hypernetwork} provides the limitations of HyperNetwork in DMG problem.

\item Section ~\ref{sec:appendix_parameters_visualization} provides the 3d visualization results of the parameters.

\item Section ~\ref{sec:appendix_implementation_detail} reports hyperparameters and training schedules of DUET.

\item Section ~\ref{sec:pseudo_code} shows the pseudo code of DUET.

\item Section ~\ref{sec:appendix_practicability} reports the practicability of the sufficient conditions.

\end{itemize}

\subsection{Limitations of HyperNetwork}
\label{sec:appendix_limitation_of_hypernetwork}
\begin{figure}[!h]
  \centering
\includegraphics[width=0.996\linewidth]{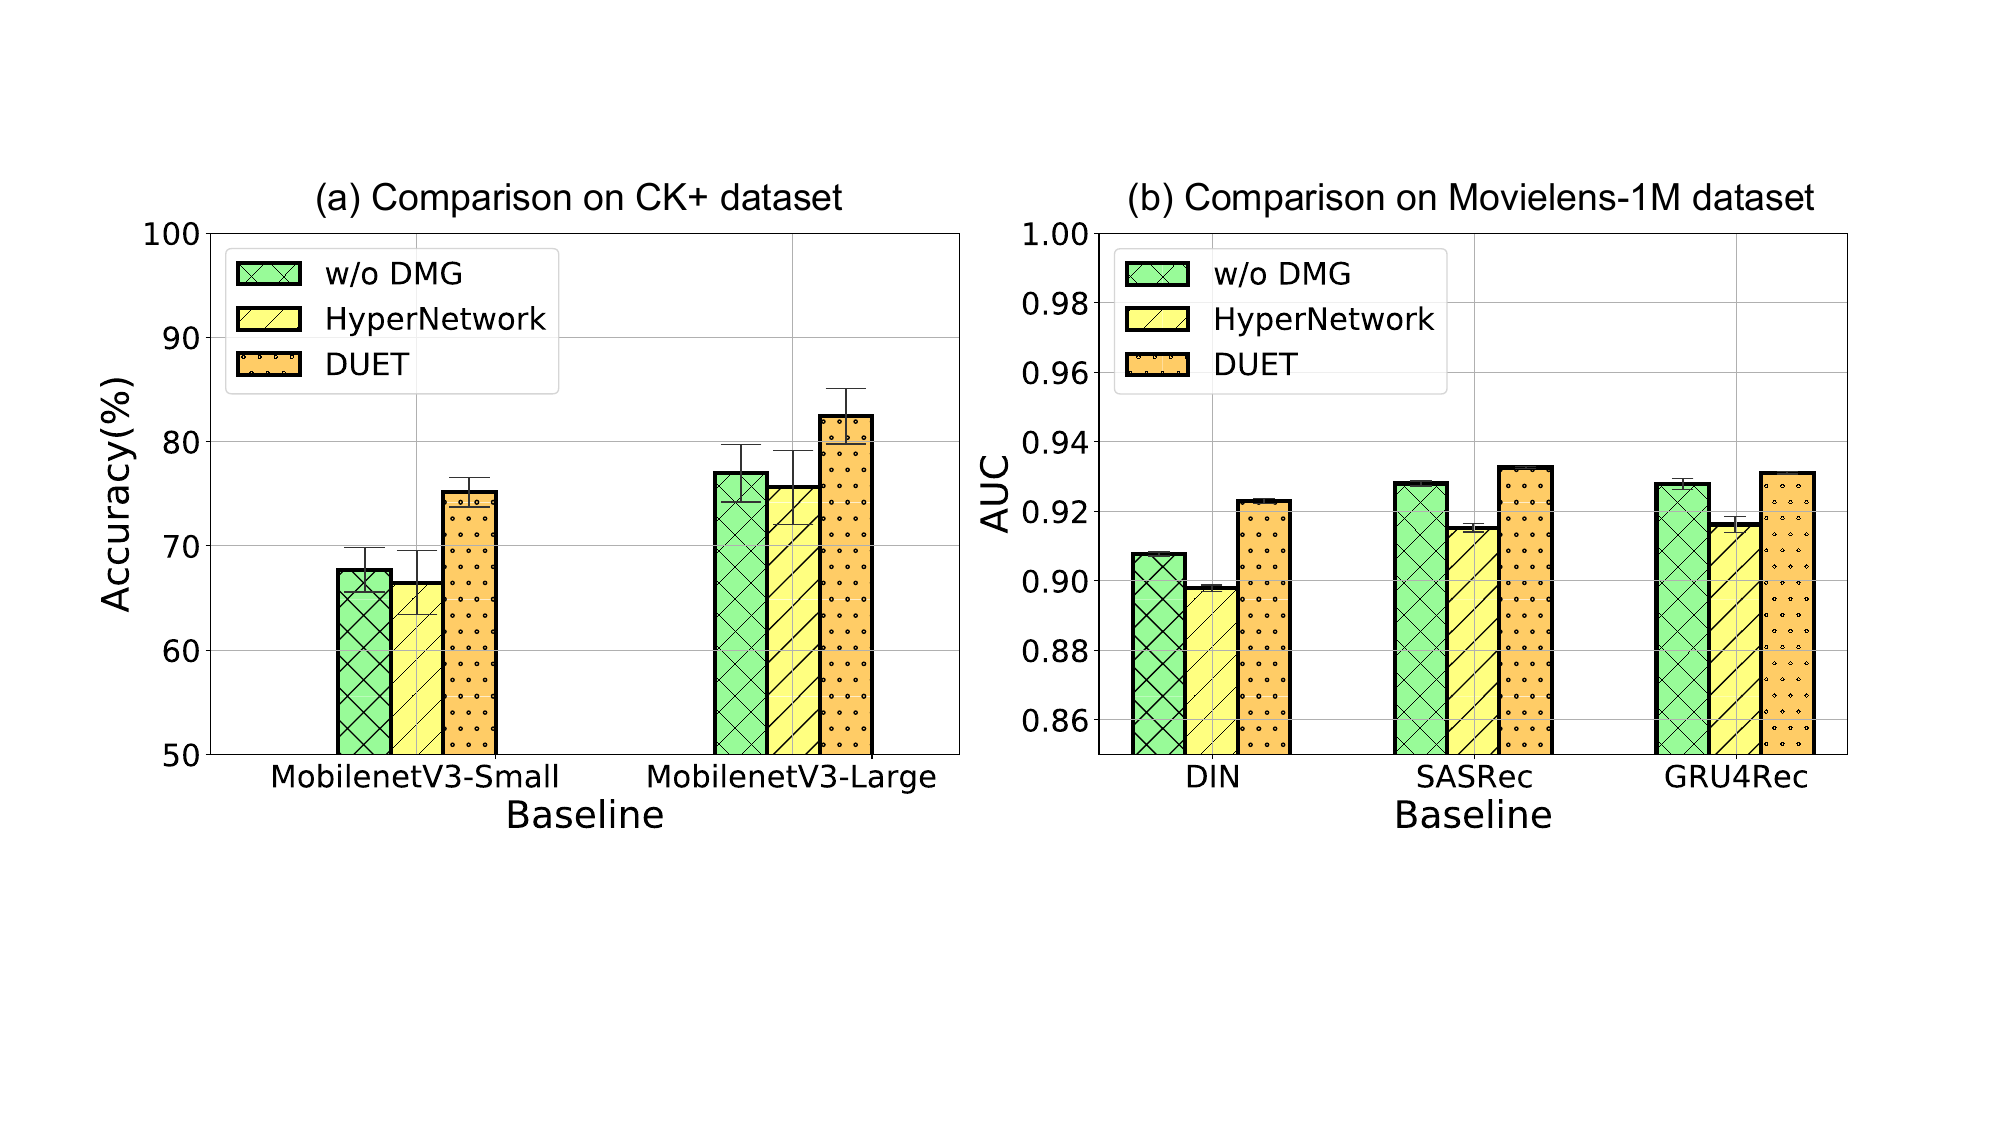}
%   \caption{Performance before and after updating the model. }
  \caption{Performance comparison between baselines, HyperNetwork and DUET on CK+ dataset and Movielens-1M dataset.}
  \label{fig:hypernetwork}
\end{figure}
Fig.\ref{fig:hypernetwork} shows that although HyperNetwork can save space when the model is stored on the device, it brings performance degradation and greater instability (\emph{i.e.}, lower standard deviation) due to the shortcomings of HyperNetwork we have discussed above. Because HyperNetwork cannot be directly applied, we have to make improvements based on HyperNetwork to adapt to the device-cloud collaboration environment. The results show that the proposed DUET significantly outperforms baselines and HyperNetwork.
\subsection{Parameters Visualization}
\label{sec:appendix_parameters_visualization}
\begin{figure}[!h]
    \centering
    \begin{subfigure}[t]{0.234\textwidth}
          \centering
        \includegraphics[width=0.98\linewidth]{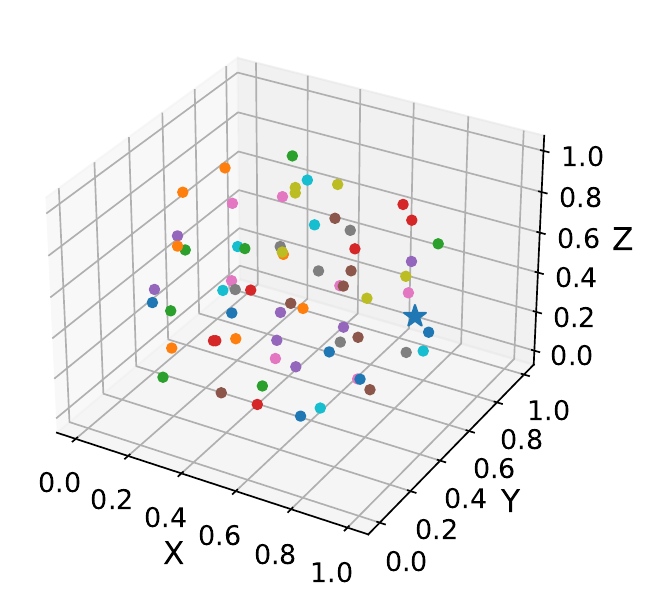}
            \caption{Visualization of convolutional layers.}
            \label{fig:tsne_vis_a}
    \end{subfigure}
    \begin{subfigure}[t]{0.234\textwidth}
            \centering
            \includegraphics[width=0.98\linewidth]{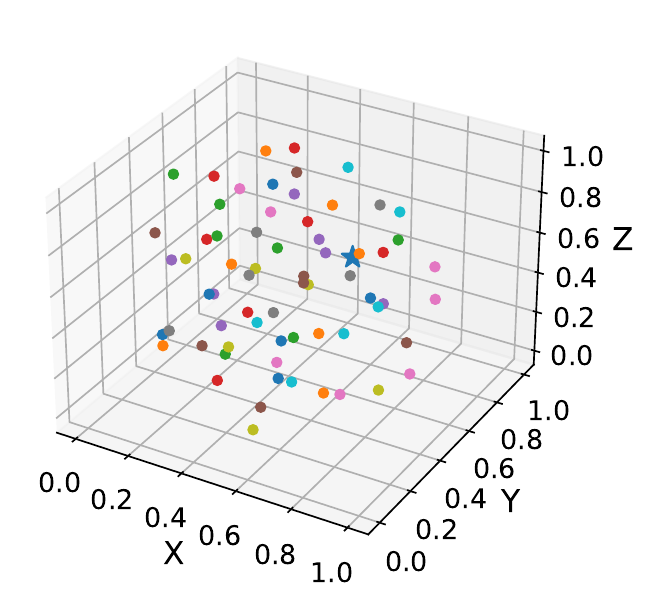}
            
            \caption{Visualization of fully connected layers.}
            \label{fig:tsne_vis_b}
    \end{subfigure}
    \caption{The 3d visualization results of the dynamic layer of UMN under DUET and the fixed layers of the primary model using the t-SNE method~\cite{van2008visualizing}.}
    \label{fig:tsne_vis}
%\vspace{-0.2cm}
\end{figure}
We choose MobilenetV3-Large as the baseline, and use t-SNE to reduce and standardize the dynamic adaptive model parameters generated by DUET and the fixed model parameters of the baseline. The former is represented by dots in various colors, and the latter is represented by large-sized asterisks. Fig.~\ref{fig:tsne_vis} shows the dimensionality reduction results of the last convolutional layer and the last fully connected layer. The experimental results show that DUET can generate adaptive parameters for the convolutional and fully connected layers according to the data of different distributions.

\subsection{Hyperparameters and Training Schedules}
\label{sec:appendix_implementation_detail}

% Table~\ref{tab:hyperparameters_and_training_schedule} shows the hyper-parameter setting on three datasets.
We summarize the hyperparameters and training schedules of DUET on the three datasets in Table~\ref{tab:hyperparameters_and_training_schedule}.
\begin{table}[!h]
    \caption{Hyperparameters and training schedules of DUET.}
    \centering
    % \resizebox{mm}{20.5mm}{
% \scalebox{0.85}{
 \resizebox{0.4\textwidth}{!}{
    \begin{tabular}{c|c|c}
    \toprule[2pt]
    % \multicolumn{2}{c|}{Method} & MetaStabilizer & Accuracy(\%) \\
    Dataset & Parameters & Setting \\ 
    \midrule[1.5pt]
    \multirow{9}{*}{CK+} & GPU & Tesla V100 \\ \cline{2-3}
    \multirow{9}{*}{} & Optimizer & Adam\\ \cline{2-3}
    \multirow{9}{*}{} & \makecell[c]{Learning rate} & 0.001\\ \cline{2-3}
    \multirow{9}{*}{} & \makecell[c]{Weight decay} & 0.0005 \\ \cline{2-3}
    \multirow{9}{*}{} & \makecell[c]{Batch size} & 128 or 64 \\ \cline{2-3}
    \multirow{9}{*}{} & \makecell[c]{Image shape} & 224×224×3 \\ \cline{2-3}
    \multirow{9}{*}{} & \makecell[c]{the Dimension of $z$} & 1×64 \\ \cline{2-3}
    \multirow{9}{*}{} & $\gamma$ & 1 \\ 
    \cline{2-3}
    \multirow{9}{*}{} & $\tau$ & 1 \\ 
\midrule[1.5pt]
    \multirow{8}{*}{\makecell[c]{Movielens-1M}} & GPU & Tesla V100 \\ \cline{2-3}
    \multirow{8}{*}{} & Optimizer & Adam\\ \cline{2-3}
    \multirow{8}{*}{} & \makecell[c]{Learning rate} & 0.001\\ \cline{2-3}
    \multirow{8}{*}{} & \makecell[c]{Batch size} & 512 \\ \cline{2-3}
    \multirow{8}{*}{} & \makecell[c]{Sequence length} & 30 \\ \cline{2-3}
    \multirow{8}{*}{} & \makecell[c]{the Dimension of $z$} & 1×64 \\ \cline{2-3}
    \multirow{8}{*}{} & $\gamma$ & 1 \\ \cline{2-3}
    \multirow{8}{*}{} & $\tau$ & 1 \\ 
\midrule[1.5pt]
    \multirow{8}{*}{\makecell[c]{Movlenes-100k}} & GPU & Tesla V100 \\ \cline{2-3}
    \multirow{8}{*}{} & Optimizer & Adam\\ \cline{2-3}
    \multirow{8}{*}{} & \makecell[c]{Learning rate} & 0.001\\ \cline{2-3}
    \multirow{8}{*}{} & \makecell[c]{Batch size} & 512 \\ \cline{2-3}
    \multirow{8}{*}{} & \makecell[c]{Sequence length} & 30 \\ \cline{2-3}
    \multirow{8}{*}{} & \makecell[c]{the Dimension of $z$} & 1×64 \\ \cline{2-3}
    \multirow{8}{*}{} & $\gamma$ & 1 \\ \cline{2-3}
    \multirow{8}{*}{} & $\tau$ & 1 \\ 
     \bottomrule[2pt]
    \end{tabular}
    }
    % }
    % }
    \label{tab:hyperparameters_and_training_schedule}
\end{table}

\subsection{Pseudo Code of DUET}
\label{sec:pseudo_code}
Algorithm~\ref{alg:pseudo_code} shows the pseudo code of DUET.
  % Use Input in the format of Algorithm
% \renewcommand{\algorithmicensure}{\textbf{Output:}} % Use Output in the format of Algorithm

\begin{algorithm}[!h]
\begin{flushleft}
% \SetAlgoLined
  \caption{DUET:  A Tuning-Free Device-Cloud Collaborative Parameters Generation Framework}
   % \textbf{Stage I:}{~\colorbox{gray!30}{$\rhd$~\emph{Train the Trunk Network}}\\
   % \textbf{Stage I:}{~\colorbox{gray!30}{$\rhd$~\emph{Cloud Model}}\\ 
    \textbf{Input}: 
    \emph{Device} $\rightarrow$ \emph{Cloud}: history samples $\mathcal{S}_{H^{(i)}}, y^{(j)}_{H^{(i)}}\}_{j=1}^{\mathcal{N}_{H^{(i)}}}$ and real-time samples $\mathcal{S}_{R^{(i)}}=\{x^{(j)}_{R^{(i)}}\}_{j=1}^{\mathcal{N}_{R^{(i)}}}$; \\
    \textbf{Output}: \emph{Cloud} $\rightarrow$ \emph{Device}: personalized classifier parameters $\Theta_l^c$. \\
    \textbf{Initialization}: Randomly initialize the parameters $\Theta_g^b$, $\Theta_g^c$ and $\Theta_p$;
     \Repeat {Convergence}{
     \If{global model or PPG in DUET have not trained} {
           Randomly sample a minibatch;\\
           Train primary cloud model $\mathcal{M}_{g}(\{\mathcal{S}_{H^{(i)}}\}_{i=1}^{\mathcal{N}_d};\Theta_g)$ with $\mathcal{S}_{H^{(i)}}$ using Eq.(2); \\
           Train PPG g($\{\mathcal{S}_{H^{(i)}}\}_{i=1}^{\mathcal{N}_d};\Theta_p$) with with $\mathcal{S}_{H^{(i)}}$ using Eq.(7);
           }
          }
      Uploading real-time samples $\mathcal{S}_{R^{(i)}}=\{x^{(j)}_{R^{(i)}}\}_{j=1}^{\mathcal{N}_{R^{(i)}}}$ to cloud;
      Generating dynamic classifier parameters $\Theta_l^c$;\\
  \Return{local device model $\mathcal{M}_{d^{(i)}}(\cdot; \Theta_g^b, \Theta_l^c)$ }.
\label{alg:pseudo_code}
\end{flushleft}
\end{algorithm}

\subsection{Practicability Analysis.}
\label{sec:appendix_practicability}

In the recommendation task, such as e-commerce recommendation or news recommendation, it is necessary to deploy a lightweight model with DMG for recommendation on a smart device, which needs to do on-device reranking or other recommendation tasks according to the user's real-time click sequence. Similarly, with the vigorous development of VR and digital virtual humans, it is also necessary to deploy lightweight models on smart devices such as mobile phones and VR devices to better apply the models in various scenarios. In these scenarios,
 our proposed DUET can be boost the DMG for better on-device learning.
